# Supplementary material for: A Stochastic Quasi-Newton Method for Large-Scale Nonconvex Optimization with Applications
Source: arXiv:1912.04456 source file (2019-12-10)
Supplement: Supplementary file 1 [file SUPPLEMENTARY_SQN.pdf]

# Supplementary Material: A Stochastic Quasi-Newton Method for Large-Scale Nonconvex Optimization with Applications

H. Chen, H. C. Wu, *Member, IEEE*, S. C. Chan, *Member, IEEE*, and W. H. Lam, *Senior Member, IEEE*

## I. Introduction

In this supplementary material, we shall evaluate the performance of various algorithms using a real *scene* dataset in Section II. A study of the sensitivity of various parameters for the proposed approach in solving the logistic regression (LR) and Bayesian logistic regression (BLR) will be presented in Section III. In Section IV, we shall compare the complexity of various algorithms. In Section V, we shall evaluate the performance of various algorithms using the nonconvex support vector machine (SVM).

## II. Numerical experiment using a real *scene* dataset

In this section, we compare the proposed stochastic damped regularized Broyden–Fletcher–Goldfarb–Shanno (Sd-REG-LBFGS) algorithm with other state-of-the-art algorithms using a real dataset: *scene* dataset [1]. It can be obtained at http://mulan.sourceforge.net/datasets-mlc.html. We employed a real *scene* dataset with 2000 samples for 5-fold cross validation and 50 Monte Carlo runs. Each image has 294 features and up to 6 scene labels: *beach*, *sunset*, *fall-foliage*, *field*, *mountain* and *urban*. To form the binary classification problems, we simply group *beach*, *sunset* and *fall-foliage* as a new category which has the label $z=1$. We further group the remaining categories with the label value $z=0$. The performance of various algorithms will be evaluated in terms of the norm of the gradient (NOG) and the classification accuracy (ACC). The NOG for LR is defined as follows:

$$\mathrm{NOG} = \left\| \frac{1}{N} \sum_{n=1}^{N} [z_n - \sigma(\theta^T x_n)] x_n \right\|. \quad \text{(S1)}$$

Moreover, the exact gradient of the objective function in BLR can be calculated as follows:

$$\nabla_\theta \mathcal{L}(\theta) = \frac{1}{N} \sum_{n=1}^{N} \{ [z_n - \sigma(\theta^T x_n)] x_n + \frac{1}{2} \sigma(\theta^T x_n) \cdot \sigma(-\theta^T x_n) [1 - 2\sigma(\theta^T x_n)] x_n x_n^T S x_n \} + S_0^{-1}. \quad \text{(S2)}$$

Hence, the NOG for BLR is defined as $\mathrm{NOG} = \|\nabla_\theta \mathcal{L}\|$. Lower NOG indicates the better convergence of an algorithm to a stationary point. The classification accuracy is given as

$$ACC = \frac{TP+TN}{TP+FN+FP+FN}. \quad \text{(S3)}$$

The decision rules for class prediction are given as

$$\text{if } \sigma(\hat{\theta}^T x_n) \geq 0.5, \text{then } z_n = 1, \text{else } z_n = 0. \quad \text{(S4)}$$

The following scanerios are considered for the *scene* dataset:

S3. Performance of various algorithms solving Logistic Regression (LR) using a real *scene* dataset with 2000 samples and 294 variables.

S4. Performance of various algorithms solving Bayesian Logistic Regression using a real *scene* dataset with 2000 samples and 294 variables.

The following algorithms are considered for evaluation:

1. Proposed Sd-REG-LBFGS method;
2. SdLBFGS: Stochastic damped LBFGS without regularization in [3];
3. Stochastic gradient difference (SGD);
4. Stochastic approximation averaging (SAA) in [4] ;
5. Robust stochastic approximation (RSA) in [5].
6. Adam in [7].

### A. Logistic Regression

In Figs. S1(a) and S1(b), we investigate the performance of the proposed Sd-REG-LBFGS method with different batch sizes. The regularization parameter is fixed at $\gamma = 10^{-4}$ and the corresponding $\delta$ is $\delta = 1.25\gamma + 0.01$. The interval length used for averaging and LBFGS updating is set to $L = 10$. SdLBFGS, SGD, RSA, SAA and Adam are also implemented for comparison. The step sizes are all $r = 7$. We find that larger batch size generally leads to better NOG performance and classification accuracy. Both methods outperform significantly SGD, RSA, SAA and Adam. Comparing between the proposed Sd-REG-LBFGS method and the SdLBFGS, while our proposed method outperforms SdLBFGS in NOG, they have nearly the same ACC performance.

Fig. S2(a) reports the effect of memory size on NOG performance using the proposed Sd-REG-LBFGS method and SdLBFGS. SGD, RSA , SAA and Adam are also implemented for comparison. Fig. S2(b) shows the corresponding ACC performance. In this experiment, the batch size is set to $m=50$. Both the NOG and classification performance generally improve when the memory size increases. However, these improvements are rather small beyond $M=8$. Moreover, our method shows better performance in NOG comparing to SdLBFGS, while its ACC is comparable with SdLBFGS under this setting. Since there is rather small improvement as memory increases beyond $M=8$ for our method, one can choose a relatively small memory size (say $M=8$) to reduce the computational time

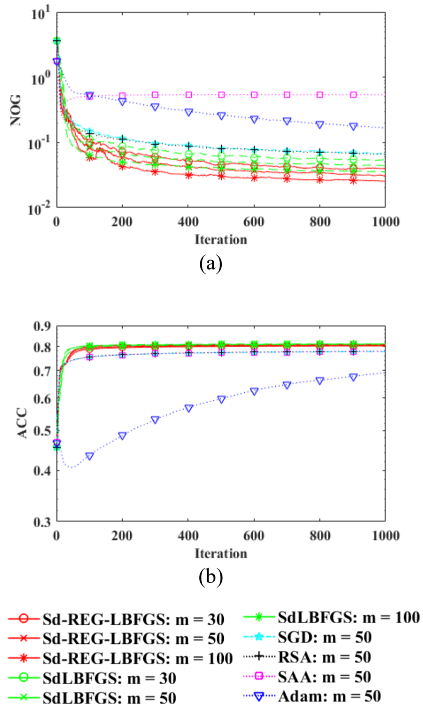


Fig. S1: The (a) Norm of Gradient (NOG) and (b) Classification Accuracy (ACC) of logistic regression solved using various algorithms with different batch sizes averaged over 50 Monte Carlo simulations. The *scene* dataset is used.

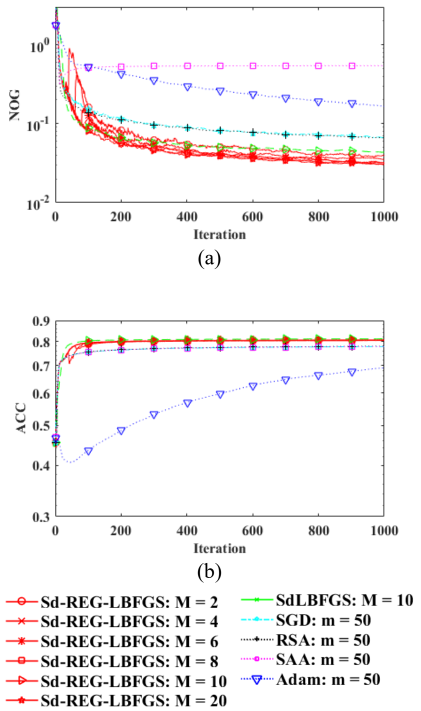


Fig S2: The (a) NOG and (b) ACC of logistic regression solved using various algorithms with different memory sizes averaged over 50 Monte Carlo simulations. For comparison, SdLBFGS, SGD, RSA, SAA and Adam are implemented. The *scene* dataset is used.

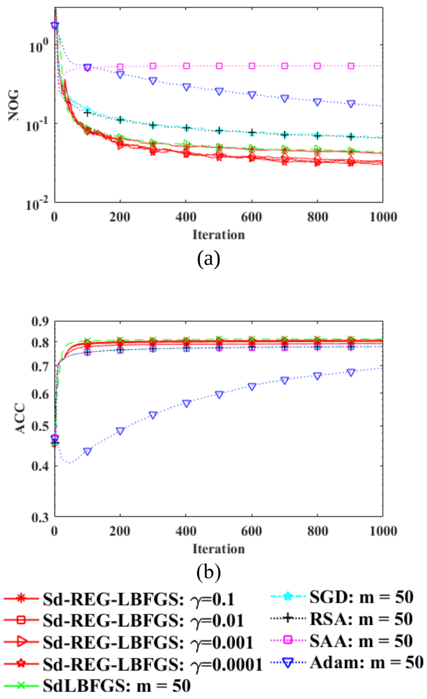


Fig. S3: The effect of regularized parameter $\gamma$ on the (a) NOG and (b) ACC of logistic regression solved using the proposed Sd-REG-LBFGS. For comparison, SdLBFGS, SGD, RSA, SAA and Adam are implemented. The *scene* dataset is used.

without sacrificing performance. Since the ACC of the proposed Sd-REG-LBFGS method is similar to that of the SdLBFGS under this setting, we shall further evaluate the two algorithms under other settings in Section V.C of the manuscript.

Next, we investigate the effect of the regularization parameter $\gamma$ on the performance of our proposed algorithm in the Figs. S3(a) and S3(b). We study the effect of the regularization parameter on the proposed Sd-REG-LBFGS algorithm in terms of NOG and ACC, respectively. The following values of $\gamma = 10^{-1}, 10^{-2}, 10^{-3}, 10^{-4}$ are employed. We can see that the proposed approach performs better in terms of NOG and ACC. We notice the small amount of regularization imposed in the proposed Sd-REG-LBFGS method generally lead to better NOG than the SdLBFGS while its ACC is similar to SdLBFGS.

*B. SDVBI for Bayesian Logistic Regression*

Figs. S4(a) and S4(b) show the performance of our method with different batch sizes applied to SDVBI. From the figures, the proposed approach has shown better performance with smaller batch size and exhibits the best NOG performance, whereas its classification accuracy is comparable with SdLBFGS for larger batch size. This aligns well with the fact that the proposed approach is the regularized extension of the SdLBFGS, where the regularization helps to improve its numerical stability under insufficient sample and its performance should be similar to the SdLBFGS when there are plenty of samples. Additionally, both methods outperform the SGD, RSA, SAA and Adam algorithm.

In Figs. S5(a) and S5(b), we numerically investigate the effect of memory size $M$ on the performance of our proposed algorithm in SDVBI. In general, larger memory size gives better performance in NOG and classification accuracy. Comparing with the proposed approach with regularization disabled, SdLBFGS with the same memory settings in terms of NOG performance. When performing under smaller memory size in the early iterations, the Hessian approximation is rather crude, as the fluctuation shown in Figs. 5(a) and 5(b) in early iterations $k= 50$ and *100*. As $M$ increases beyond $M=4$, the performance improvement is rather small.

In Figs. S6(a) and S6(b), we numerically study the effect of regularized parameter on the performance of Sd-REG-LBFGS for SDVBI. Similar to Figs. S3(a) and S3(b), we notice the small amount of regularization imposed in the proposed Sd-REG-LBFGS method generally lead to better NOG than the SdLBFGS while its ACC is similar to SdLBFGS.

Overall, we find that the proposed approach performs better than other conventional algorithms in terms of NOG and ACC. This may be attributed by the small amount of regularization applied to the proposed approach, which improves the numerical stability and hence it converges closer to the stationary point (lower NOG). Meanwhile, we notice the ACC of the proposed Sd-

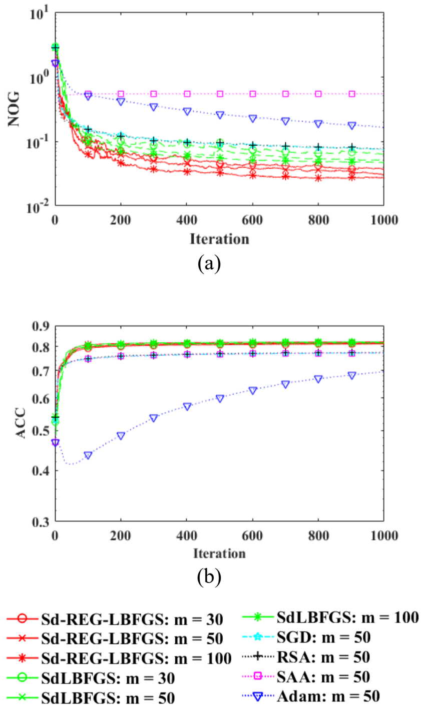


Fig. S4: The (a) NOG and (b) ACC of different algorithms with various batch sizes in solving SDVBI in Bayesian logistic regression. For comparison, SdLBFGS, SGD, RSA, SAA and Adam are included. The *scene* dataset is used.

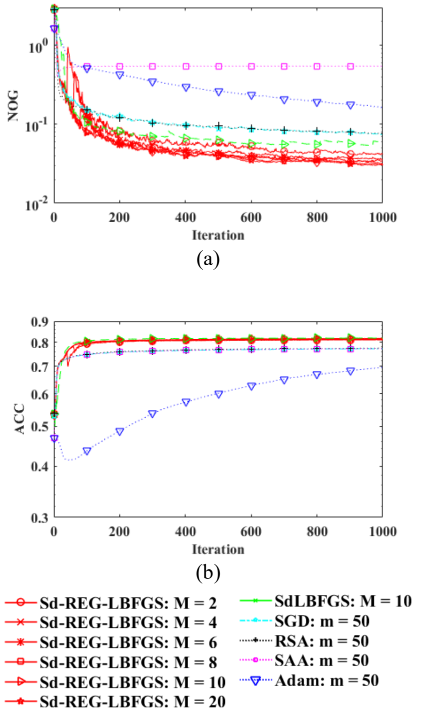


Fig. S5: The (a) NOG and (b) ACC of SDVBI in Bayesian logistic regression solved using various algorithms with different memory sizes averaged over 50 Monte Carlo simulations. For comparison, SdLBFGS, SGD, RSA, SAA and Adam are included. The *scene* dataset is used.

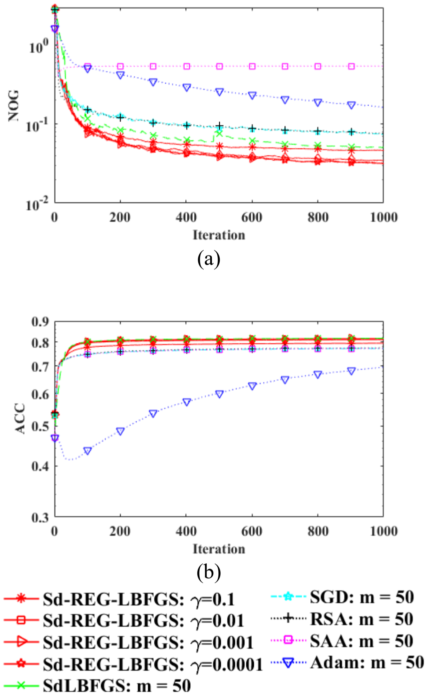


Fig. S6: The effect of regularized parameter $\gamma$ on the (a) NOG and (b) ACC of SDVBI in Bayesian logistic regression solved using the proposed Sd-REG-LBFGS. For comparison, SdLBFGS, SGD, RSA, SAA and Adam are implemented. The *scene* dataset is used.

REG-LBFGS and the Sd-LBFGS are quite similar under this setting.

## II. Sensitivity Analysis

In this section, we study the sensitivity of the proposed approach in the following parameters: i) batch size $m$, ii) Memory size $M$ and regularization parameter $\gamma$ using the following four scenarios:

S1. Performance of various algorithms solving LR using synthetic data of 5000 samples and 50 variables.

S2. Performance of various algorithms solving LR using a real *scene* dataset with 2000 samples and 294 variables.

S3. Performance of various algorithms solving BLR using synthetic data of 5000 samples and 50 variables.

S4. Performance of various algorithms solving BLR using a real *scene* dataset with 2000 samples and 294 variables.

For each scenario, we have conducted 50 Monte Carlo simulations, in which 5-fold cross validation is adopted. The maximum number of iterations is chosen to be 1000, which is sufficient for all algorithms to converge. We compare the proposed approach with the Stochastic Damped Limited Memeory Broyden–Fletcher–Goldfarb–Shanno (SdLBFGS), Stochastic Gradient Difference (SGD), Robust Stochastic Average Gradient (RSA), Stochastic Approximation Averaging (SAA) and Adam Algorithms.

### *A.* Batch size

In this subsection, we evaluate the performance of various algorithms under batch sizes $m = 5,10,30,50,100,200$ for the scenarios with synthetic dataset and $m = 5,10,20,30,50,100$ for the scenarios with *scene* dataset.

### A.1 Logistic regression (scenarios 1 and 2)

Fig. S7(a) and S7(b) shows the NOG and ACC respectively of all algorithms using different batch sizes for the synthetic dataset. It can be seen that the proposed Sd-REG-LBFGS performs the best in NOG and ACC among the different algorithms. In particular, we find that the additional regularization imposed on the proposed approach is particularly useful to deal with small batch sizes $m = 5,10$, where the proposed approach is able to maintain numerical stability and attains good NOG and ACC performance but the conventional SdLBFGS suffers from ill-conditioning of the Hessian approximation matrix. Since the SdLBFGS becomes ill-conditioned in some of the 50 Monte Carlo simulations, we only take averages of those that do not suffer from ill-conditioning. We find that the proposed approach still performs better than the SdlBFGS despite the fact that only the better Monte Carlo simulations are counted for the SdLBFGS. Similar conclusions are

drawn for the evaluation using the real scene dataset as shown in Figs. S7(c) and S7(d).

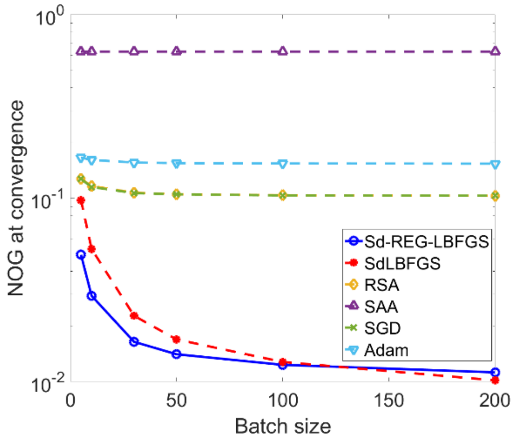


Fig. S7(a). The Norm of Gradient (NOG) of various algorithms solving logistic regression for synthetic dataset (scenario 1).

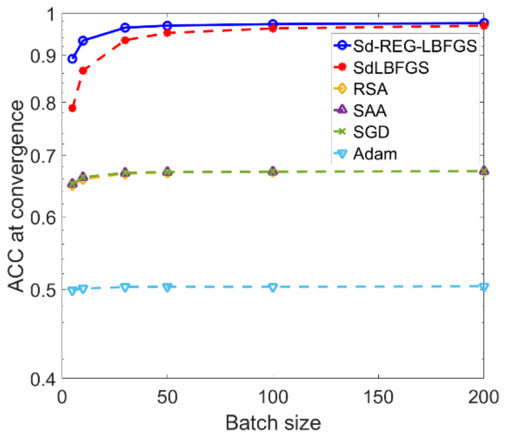


Fig. S7(b). The Classification Accuracy (ACC) of various algorithms solving logistic regression for synthetic dataset (scenario 1).

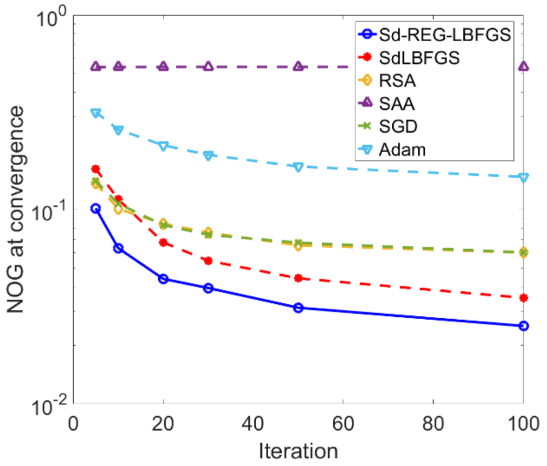


Fig. S7(c). The NOG of various algorithms solving logistic regression for the real (scene) dataset (scenario 2).

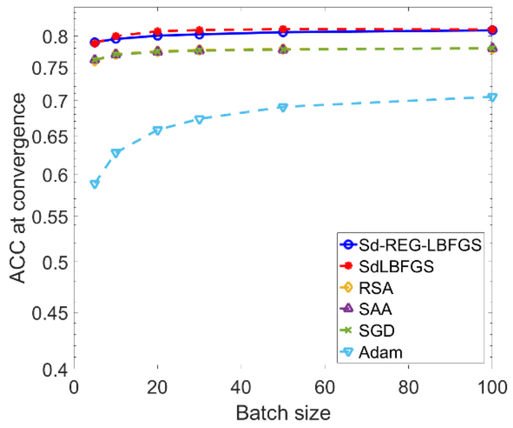


Fig. S7(d). The ACC for various algorithms solving logistic regression for the real (scene) dataset (scenario 2).

Overall, our method has the best performance and is more robust to small batch sizes due to the incorporation of regularization.

### A.2 Bayesian logistic regression (scenarios 3 and 4)

Figs. S8(a) and S8(b) show the NOG and ACC of the various algorithms in solving the Bayesian logistic regression using the synthetic dataset under different batch sizes. Overall, the proposed Sd-REG-LBFGS performs the best in NOG and ACC among the different algorithms. Moreover, its performance is generally more robust to the effect of small batch size due to the regularization imposed, whereas the conventional SdLBFGS suffers from ill-conditioning. Similarly, the proposed approach still performs better than SdLBFGS though we have only counted the Monte Carlo simulations that are not ill-conditioned for the SdLBFGS. Similar conclusions are drawn for the evaluation using the real *scene* dataset as shown in Figs. S8(c) and S8(d). Similar conclusions are drawn for the evaluation using the real scene dataset as shown in Figs. S8(c) and S8(d).

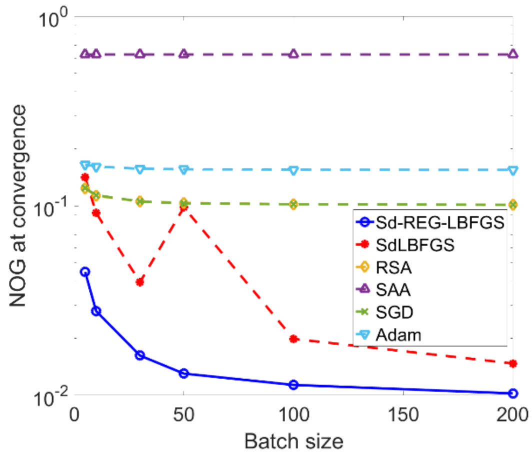


Fig. S8(a). The NOG of various algorithms solving Bayesian logistic regression for synthetic dataset (scenario 3).

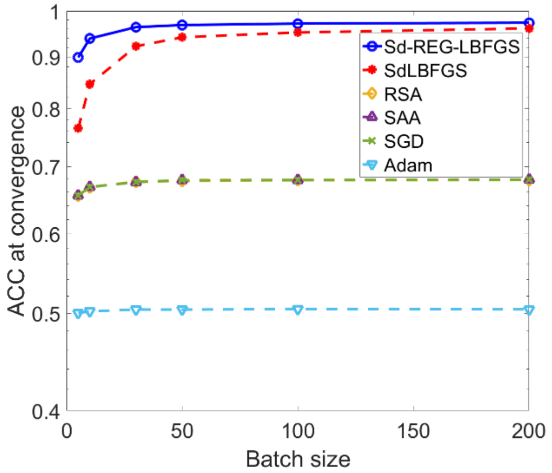


Fig. S8(b). The ACC of various algorithms solving Bayesian logistic regression for synthetic dataset (scenario 3).

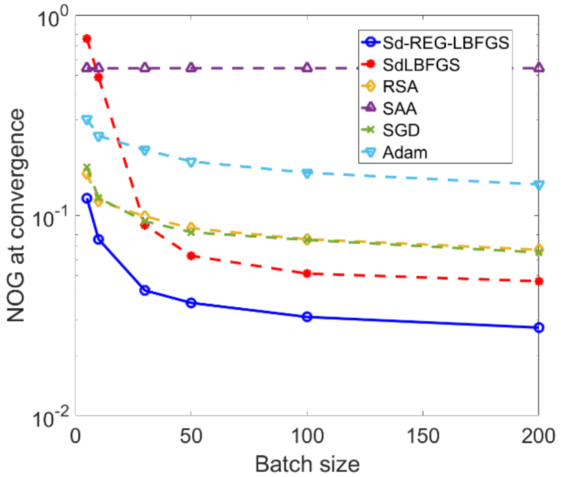


Fig. S8(c). The NOG of various algorithms solving Bayesian logistic regression for the real (scene) dataset (scenario 4).

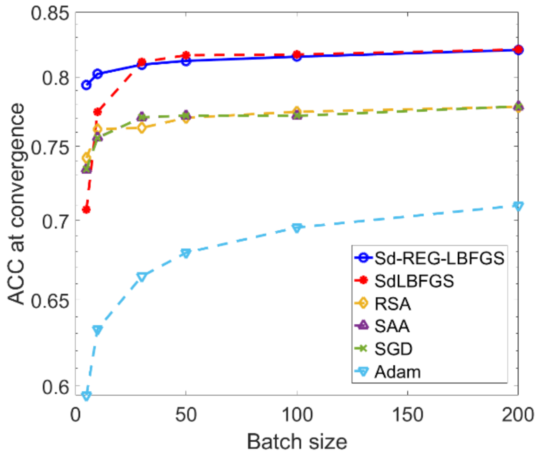


Fig. S8(d). The ACC of various algorithms solving Bayesian logistic regression for the real (scene) dataset (scenario 4).

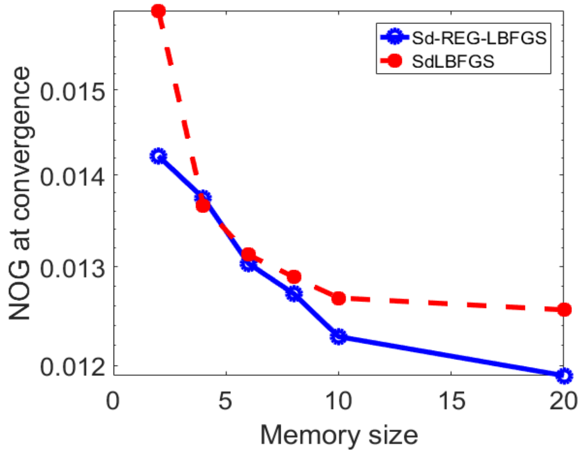


Fig. S9(a). The NOG of the proposed Sd-REG-LBFGS method and Sd-LBFGS method in solving Logistic regression for synthetic dataset (scenario 1).

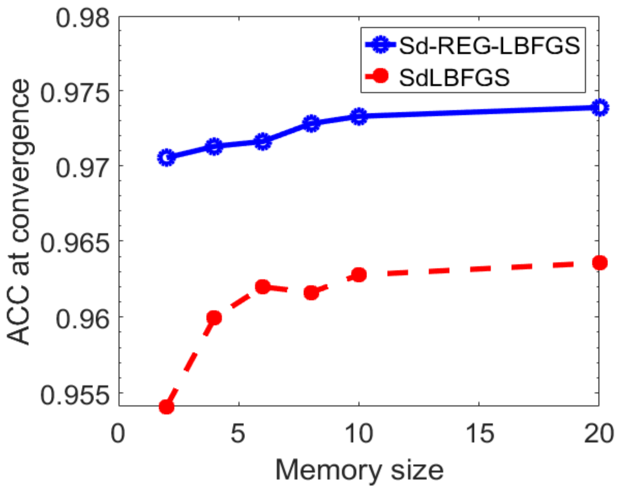


Fig. S9(b). The ACC of the proposed Sd-REG-LBFGS method and Sd-LBFGS method in solving Logistic regression for synthetic dataset (scenario 1).

From the four scenarios as depicted in Fig. S7(a) to Fig. S8(d), we can see that increasing the batch size generally improves the performance (lower norm of gradient and higher classification accuracy) of the proposed approach. Comparing with other algorithms, the performance of the proposed algorithm is less affected under small sample due to the incorporation of regularization.

*B. Memory size M*

The memory size $M$ is an algorithmic parameter unique to the proposed Sd-REG-LBFGS method and the conventional Sd-LBFGS method. Hence, we study the sensitivity of the two algorithms under different memory size $M$=2, 4, 6, 8, 10, and 20.

**B.1 Logistic regression (scenarios 1 and 2)**

More precisely, Figs. S9(a) - S9(b) show the NOC and ACC of the two algorithms for the synthetic dataset, respectively. We can see that the proposed approach generally attains better

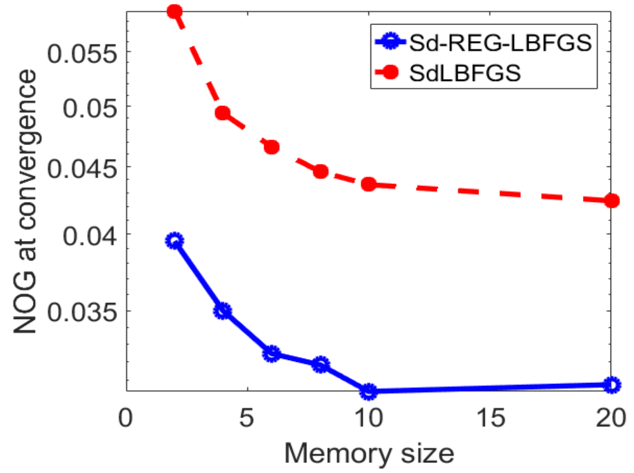


Fig. S9(c). The NOG of the proposed Sd-REG-LBFGS method and Sd-LBFGS method in solving logistic regression for the real (scene) dataset (scenario 2).

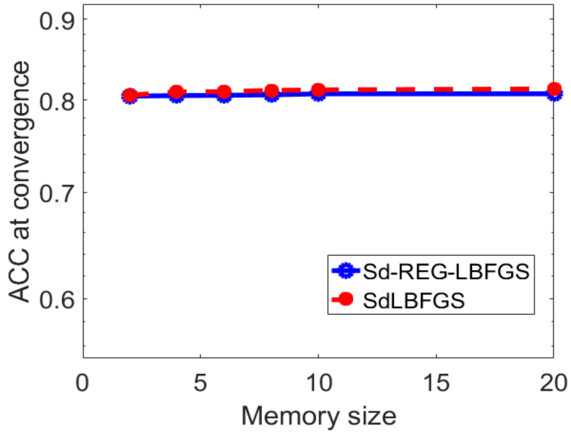


(d)

Fig. S9(d). The ACC of the proposed Sd-REG-LBFGS method and Sd-LBFGS method in solving logistic regression for the real (scene) dataset (scenario 2).

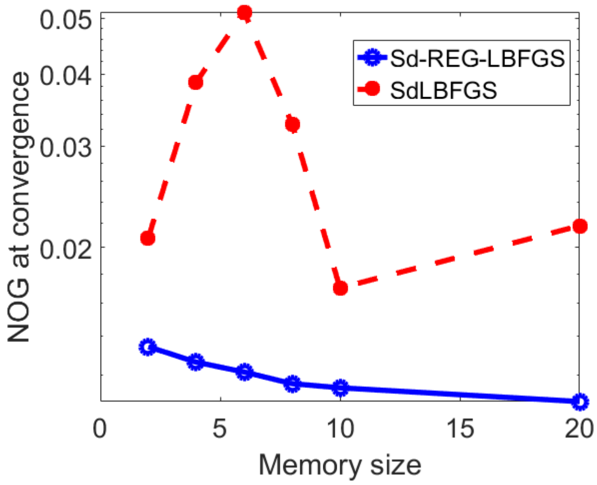


Fig. S10(a). The NOG of the proposed Sd-REG-LBFGS method and Sd-LBFGS method in solving Bayesian Logistic regression for synthetic dataset (scenario 3).

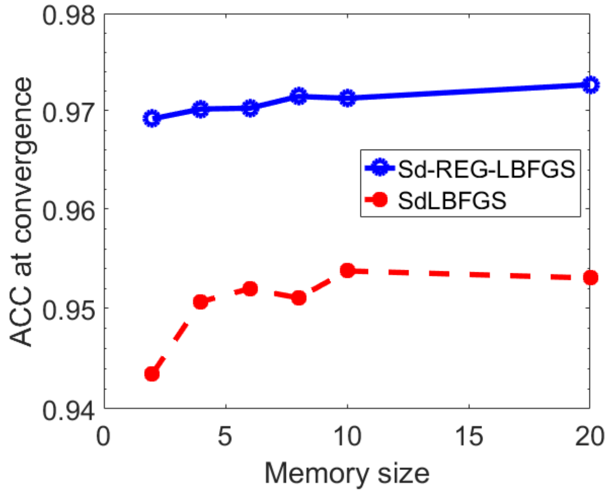


Fig. S10(b). The ACC of the proposed Sd-REG-LBFGS method and Sd-LBFGS method in solving Bayesian Logistic regression for synthetic dataset (scenario 3).

performance (lower NOG and higher ACC) comparing with the conventional SdLBFGS. On the other hand, both algorithms obtain similar ACC in the real dataset but the NOG is better for the proposed approach. Overall, we find that increasing the memory size lead to better NOG and ACC performnace, and the performance improvement is most significant when $M < 8$.

**B.2 Bayesian logistic regression (scenarios 3 and 4)**

The NOG and ACC of the proposed Sd-REG-LBFGS method and the SdLBFGS method in solving the Bayesian logistic regression using the synthetic dataset scenario are shown in Figs. S10(a) and S10(b), respectively. Overall, our method performs better than SdLBFGS in terms of NOG and ACC for different memory sizes. Moreover, the conventional SdLBFGS method has shown irregular behaviour over increasing memory size (especially in Fig S10(a)), whereas the proposed approach generally shows improvement with increasing memory size.. Similar conclusions are drawn for Figs. S10(c) and S10(d), where the NOG of the conventional SdLBFGS varies irregularly over

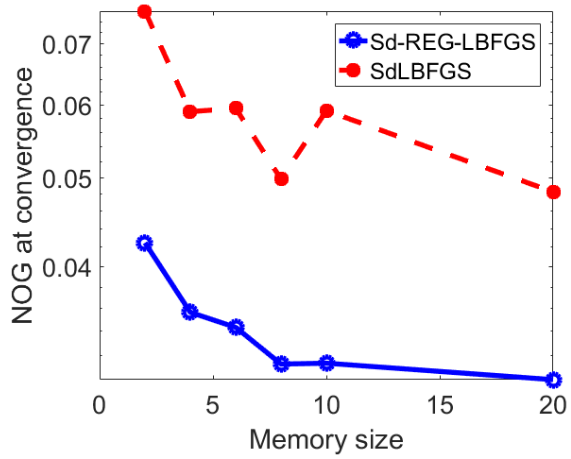


Fig. S10(c). The NOG of the proposed Sd-REG-LBFGS method and Sd-LBFGS method in solving Bayesian logistic regression for the real (scene) dataset (scenario 4).

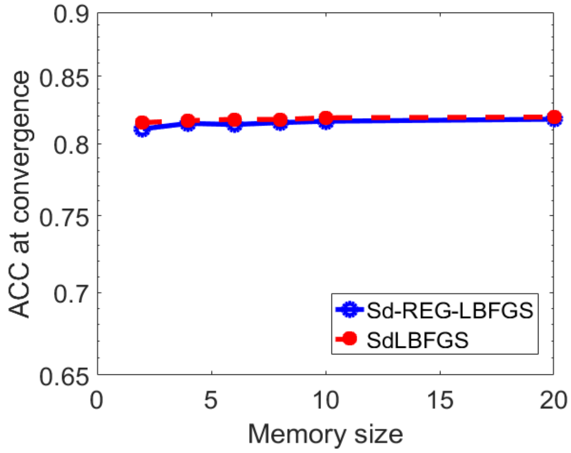


Fig. S10(d). The ACC of the proposed Sd-REG-LBFGS method and Sd-LBFGS method insolving Bayesian logistic regression for the real (scene) dataset (scenario 4).

increasing memory size and the proposed approach shows consistent improvement in performance under increasing memory size.

From the four scenarios as depicted in Figs. S9(a) to S10(d), we can see that increasing the memory size *M* generally improves the performance (lower norm of gradient and higher classification accuracy) of the proposed approach.

### C. Regularization parameter γ

Figs. S11(a) to S12(d) show the NOG and ACC for the four scanerios. We find that a small regularization parameter such as $\gamma$ from $10^{-4}$ to $10^{-2}$ generally gives better performance with lower NOG and higher ACC. However, as $\gamma$ increases from $10^{-2}$ to 1, the NOG at convergence increases evidently, which suggest further increasing the amount regularization may introduce bias to the estimation and may lead to deterioriation in estimation accuracy, which is also reflected on the decrease in ACC performance when $\gamma$ increases from $10^{-2}$ to 10.

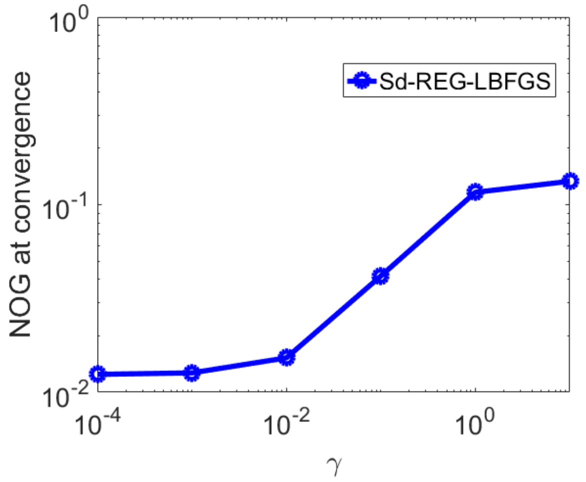


Fig. S11(a). The NOG of the proposed approach in solving logistic regression for the synthetic dataset (scenario 1).

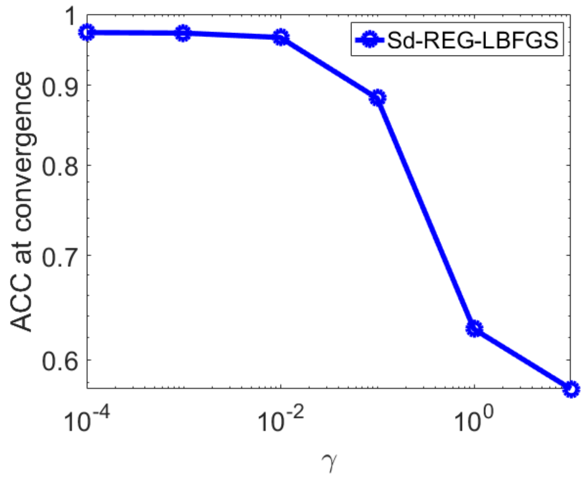


Fig. S11(b). The ACC of the proposed approach in solving logistic regression for the synthetic dataset (scenario 1).

Overall, we observe that a small regularization parameter is required to maintain the numerical stability of the optimization problem. However, the regularization introduces bias to the optimization problem and hence increasing the regularization parameter further will lead to a decrease in classification accuracy.

### D. Discussion on choice of parameters

Regarding the choice of the algorithmic parameters including the batch size *m*, memory size *M* and the regularization parameter $\gamma$, we observe a choice of *m=100* serves the best for most algorithms under the datasets we have considered. For the proposed Sd-REG-LBFGS method and the Sd-LBFGS method, a memory size of *M=8* will suffice. Beyond these values, the performance improvement is not so significant. Moreover, the complexity and computational time increases with the two parameters and hence it is desirable to keep them as small as possible. Small amount of regularization, such as $\gamma = 10^{-4}$, is fair enough to further reduces the fluctuations under sufficient samples.

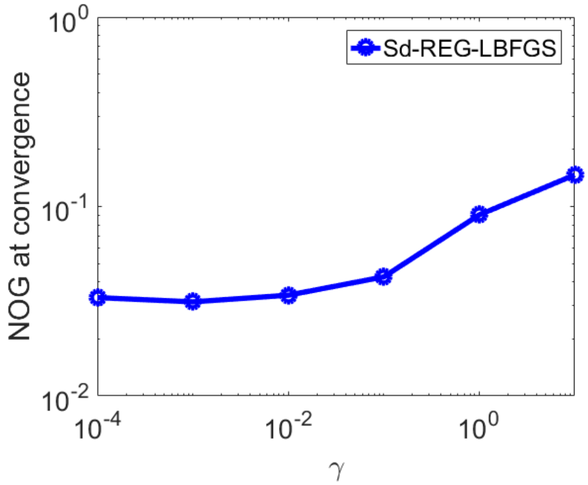


Fig. S11(c). The NOG of the proposed approach in solving logistic regression for the real (scene) dataset (scenario 2).

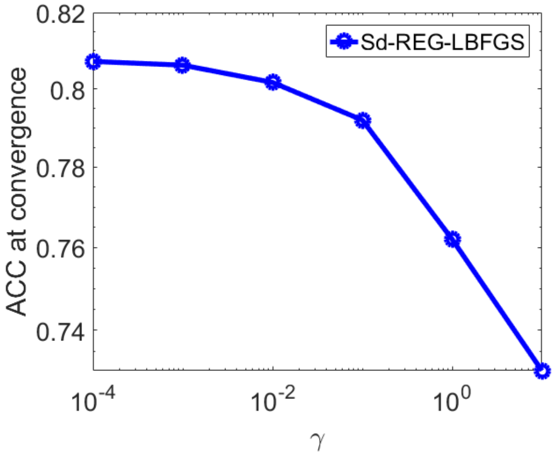


(d)

Fig. S11(d). The ACC of the proposed approach in solving logistic regression for the real (scene) dataset (scenario 2).

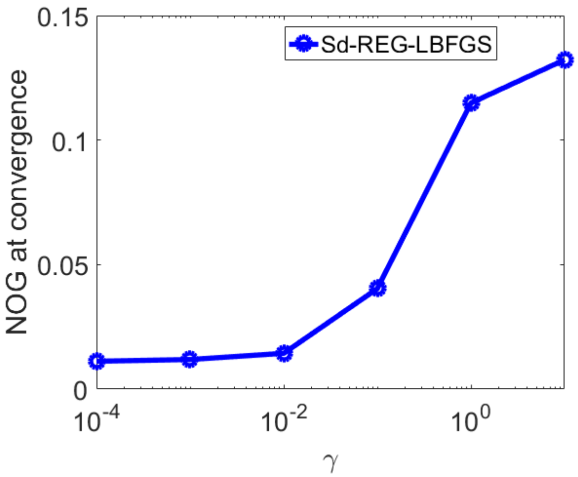


Fig S12(a). The NOG of the proposed approach solving logistic regression for the synthetic dataset (scenario 3).

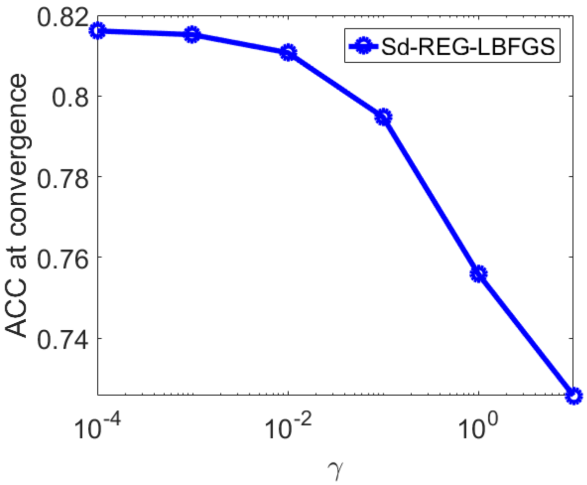


Fig S12(b). The ACC of the proposed approach solving logistic regression for the synthetic dataset (scenario 3).

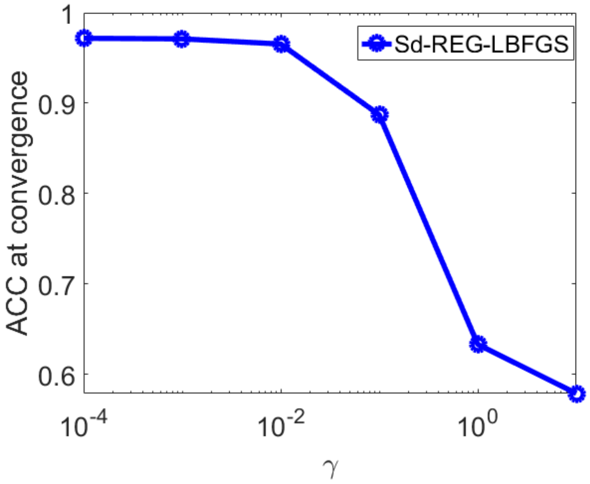


Fig S12(c). The NOG of the proposed approach solving Bayesian logistic regression for the real (scene) dataset (scenario 4).

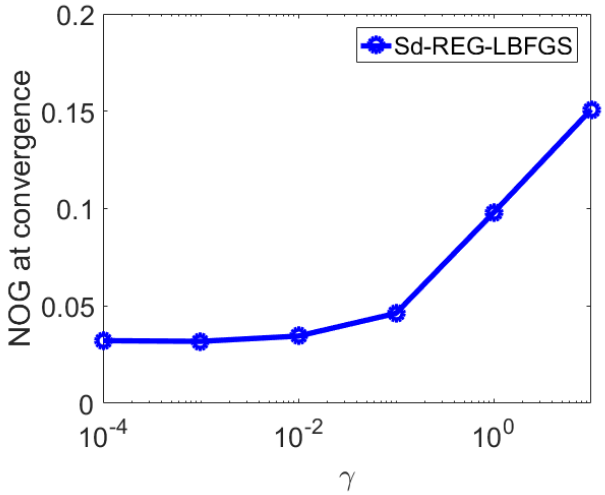


Fig S12(d). The ACC of the proposed approach solving Bayesian logistic regression for the real (scene) dataset (scenario 4).

## IV. Complexity Analysis

In this section, we study the complexity of the proposed algorithm. The complexity of various algorithms in terms of number of gradient calls and averaged complexity are summarized in Tables S1 and S2, respectively. The number of gradient calls in Table S1 are obtained from $T \cdot L$ iterations, where $T$ is an integer and L is the interval length. The complexity of each gradient calculation is $O(h)$. $\tau$ is the interval length of the iterates for weight averaging.

It can be seen from Table S1 that our method has much fewer gradient calls than SdLBFGS. Hence, our method will have its advantage over SdLBFGS in problems with much complicated gradient calculations, i.e., for large $h$, our method will be faster than SdLBFGS. Moreover, as is studied numerically, our method performs better than SdLBFGS in small batch size and requires fewer gradient evaluations to achieve the same classification performance as SdLBFGS. This has further reduced the

Table S1 Number of gradient calls of various algorithms in $T \cdot L$ iterations

| Sd-REG-LBFGS | SdLBFGS | SGD | RSA | SAA | Adam |
|---|---|---|---|---|---|
| $TLm + 2(T-1)m$ | $3TLm$ | $TLm$ | $TLm$ | $TLm$ | $TLm$ |

Table S2 Complexity of various algorithms per iteration

| Sd-REG-LBFGS | SdLBFGS | SGD | RSA | SAA | Adam |
|---|---|---|---|---|---|
| $O(mh + d^2 + \frac{d^3 + 2mh}{L})$ | $O(3mh + d^2)$ | $O(mh)$ | $O(\tau + mh)$ | $O(mh + TL)$ | $O(mh + m)$ |

complexity of our method under the same performance with SdLBFGS.

## V. NONCONVEX SVM

In this section, we continue our study on the application of our proposed method to nonconvex SVM, where the objective function is:

$$\frac{1}{N}\sum_{i=1}^{N}\{1 - \tanh(z_i\theta^T x_i)\} + \lambda\|\theta\|^2 , \qquad (S6)$$

and $x_i$ are observations, $z_i$ are the labels and $\theta$ contains the parameters to be estimated. The real *scene* dataset [1] is employed. Moreover, SdLBFGS, SGD, RSA, SAA and Adam are implemented for comparison. We employed 2000 samples with 5-fold cross validation and 50 Monte Carlo runs. The decision rule for this SVM in the testing dataset is as follows:

$$z_i = \text{sign}(\hat{\theta}^T x_i) , \qquad (S7)$$

where $\text{sign}(u) = 1$ for $u > 0$ or -1 otherwise. The regularization parameter is fixed at $\gamma = 10^{-4}$ and the corresponding $\delta$ is $\delta = 1.25\gamma + 0.01$. The interval length $L$ used for averaging and LBFGS updating is set to 10. For Sd-REG-LBFGS and SdLBFGS, their memory sizes are both set to 10. The step sizes are all $r = 7$. We choose a batch size of $m = 10$.

To illustrate the usefulness of regularization and damped BFGS scheme in stochastic LBFGS, we compare the proposed stochastic damped regularized LBFGS (Sd-REG-LBFGS) method with Sd-LBFGS (no regularization) and SLBFGS (no damping). Since soft-margin SVM is renowned for its good performance, it can be seen that from Fig. S13(b) that all algorithms perform comparably well in terms of classification accuracy (ACC). However, we can see from Fig. S13(a) that the proposed approach attains the lowest NOG, which suggests it converge closest to the stationary point. This suggest the new regularization scheme employed in the proposed approach further improves the performance of the stochastic damped LBFGS. Moreover, the damped BFGS scheme helps to improve the performance of the LBFGS under non-convex problems, which contributes to the better performance of the Sd-REG-LBFGS and Sd-LBFGS.

In general, the proposed approach can also be applied to non-convex problems such as neural network or the problems reported in [3] and [6] and it can help to tackle ill-conditioning of the Hessian under problems with insufficient samples.

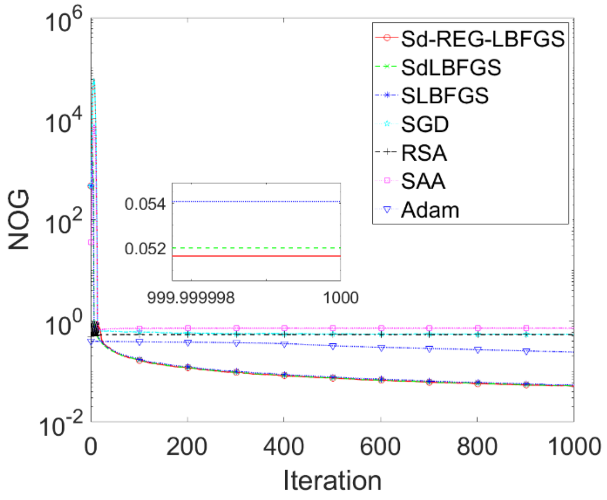


Fig. S13(a) The NOG of SVM solved using various algorithms averaged over 50 Monte Carlo simulations.

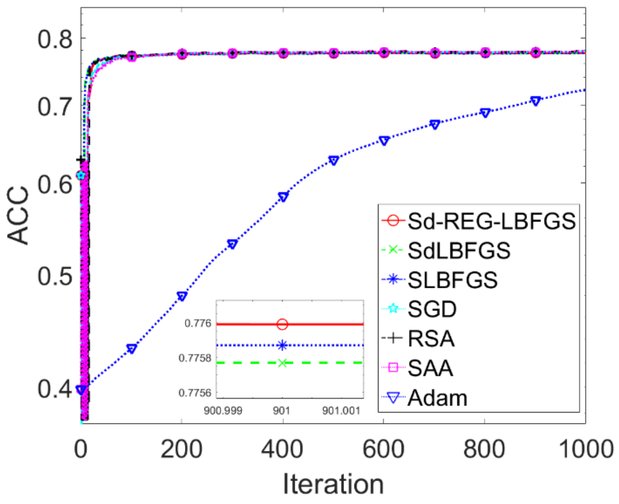


Fig. S13(b) The ACC of SVM solved using various algorithms averaged over 50 Monte Carlo simulations.

## REFERENCES


[1] M.R. Boutell, J. Luo, X. Shen, and C.M. Brown, "Learning multi-labelscene classiffication," *Pattern Recognition*, vol. 37, no. 9, pp. 1757-1771, 2004..

[2] C. Dang and G. Lan, "Stochastic Block Mirror Descent Methods for Nonsmooth and Stochastic Optimization,"*SIAM J. Optim.*, vol. 25, no. 2, pp. 856 - 881, 2015.

[3] X. Wang, S. Ma, D. Goldfarb, and W. Liu, "Stochastic Quasi-Newton Methods for Nonconvex Stochastic Optimization,"*SIAM J. Optim.*, vol. 27, no. 2, pp. 927 – 956, 2017.

[4] B. T. Polyak and A. B. Juditsky, "Acceleration of stochastic approximation by averaging," *SIAM J. Control Optim.*, vol. 30, no. 4, pp. 838-855, 1992.

[5] A. Nemirovski and A. Juditsky and G. Lan and A. Shapiro, "Robust Stochastic Approximation Approach to Stochastic Programming,"*SIAM J. Optim.*, vol. 19, no. 4, pp. 1574 - 1609, 2009.

[6] J. Nocedal, and S. J. Wright, *Numerical Optimization*, New York:Springer-Verlag, 1999.

[7] D. Kingma and J. Ba, "Adam: A method for stochastic optimization," in *3rd International Conference for Learning Representations*, 2015.
